# Supplementary material for: Soft Hybrid Aerial Vehicle via Bistable Mechanism
Source: arXiv:2011.00426 source file (2020-11-01)
Supplement: Supplementary file 1 [file 7_appendix.tex]

\section*{APPENDIX}
